# Supplementary material for: Flowtron: an Autoregressive Flow-based Generative Network for Text-to-Speech Synthesis
Source: arXiv:2005.05957 source file (2020-07-16)
Supplement: Supplementary file 1 [file appendix.tex]

%auto-ignore
